# Supplementary material for: VortSDF: 3D Modeling with Centroidal Voronoi Tesselation on Signed Distance Field
Source: arXiv:2407.19837 source file (2024-09-30)
Supplement: Supplementary file 1 [file supplemental.tex]

\begin{table*}[h]
   \centering
    \caption{Average photometric accuracy $PSNR$ (higher is better) obtained with our  method, NeuS 2 and Voxurf, for each of the $7$ test scenes. We highlight the \colorbox{Red!50}{\textbf{best}} and \colorbox{Yellow!50}{\underline{second}} values.}
    %\vspace*{3mm}
    \begin{tabular}{|c||c|c|c|c|c|c|c|c|c|}%|c|}
    \hline
     Method & f-cos-hx & f-jea-hx & f-opt1-hx & f-opt2-hx & f-opt3-hx & f-sho-hx & m-jea-hx & m-opt-hx & avg \\
    \hline
     NeuS2 & $27.6$ & $28.4$ & $31.9$ & $33.2$ & $30.3$ & $31.6$ & $29.7$ & $25.8$ & $30.79$ \\
     \hline
     VOXURF & $28.38$ & $29.32$ & $39.26$ & $37.34$ & $32.82$ & $36.73$ & $34.45$ & $37.57$ & $35.45$ \\
     \hline
     VortSDF & $\mathbf{28.80}$ & $\mathbf{29.90}$ & $\mathbf{39.64}$ & $\mathbf{37.48}$ & $\mathbf{32.95}$ & & & & \\
     \hline 
          
    \end{tabular}
    \label{tab:PSNR}
\end{table*}

\begin{table}[h]
    \centering
    \caption{Computational time analysis. We report number of rays processed per second at each level of discretization.}
    %\vspace*{3mm}
    \begin{tabular}{|c|c|c|c|c|c|}%|c|}
    \hline
     & Lvl 0 & Lvl 1 & Lvl 2 & Lvl 3 & Lvl 4\\
    \hline
    \hline
     Nb points & $30$K & $50$K & $126$K & $526$K & $2$M \\
    \hline
     Rays/second & $120$K & $80$K & $60$K & $40$K & $20$K \\  
    
    \hline
    \end{tabular}
    \label{tab:speed}
\end{table}
